# Supplementary material for: Efficient Global Point Cloud Alignment using Bayesian Nonparametric Mixtures
Source: arXiv:1603.04868 source file (2016-11-22)
Supplement: Supplementary file 1 [file figure.tex]

\begin{figure}
  \centering
  \begin{tikzpicture}
    \node (L0) at (0,0) {
      \includegraphics[width=0.2\columnwidth]{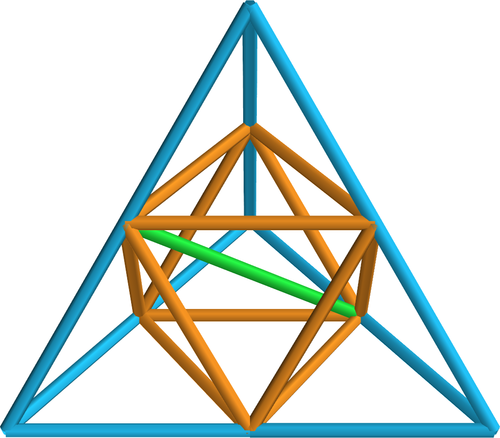}
    };
    \node[right = 1.5ex of L0] (L1) {
      \includegraphics[width=0.2\columnwidth]{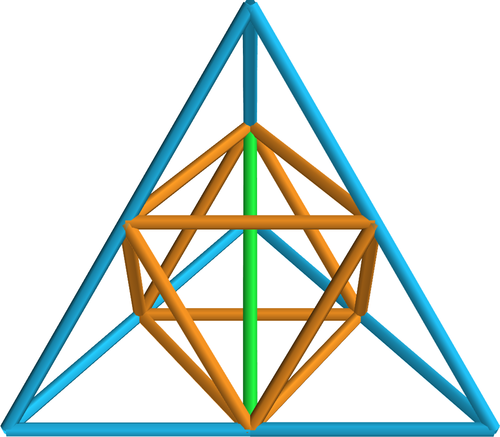}
    };
    \node[right = 1.5ex of L1] (L2) {
      \includegraphics[width=0.2\columnwidth]{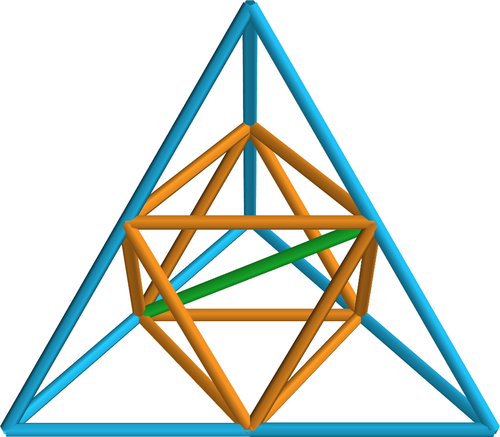}
    };
  \end{tikzpicture}
  \caption{The three subdivision patterns---due to the choice of the green edge---of a
  tetrahedron displayed in 3D. Colors designate different edge types:
  corner edges (blue) from an edge midpoint to a vertex; tie edges (orange) between two edge midpoints, running along a tetrahedron face;
and skew edges (green) between two edge midpoints, running through the inside of the tetrahedron.
%  The different colors designate corner
%edges (red), tie edges (green) and skew edges
%(blue).
\label{fig:tetrahedronSubdivision}}
\end{figure}
